# Supplementary material for: Teaching Vision-Language-Action Models to Stop Safely
Source: arXiv:2611.26239 source file (2026-11-19)
Supplement: Supplementary file 1 [file appendix_before_concision_20261117.tex]

% Appendix before the author-requested concision pass on 2026-11-17.
% Exact source fragments from commit a11058b. This is a research archive, not a manuscript input.

% SOURCE: sections/appendix.tex
\section{Appendix Outline}
\label{app:outline}
This appendix provides the complete \method procedure, detailed experimental settings, and supporting analyses for the four main research questions. It also reports computational costs and qualitative trajectory comparisons. The sections are organized as follows.

\begingroup
\small
\newcommand{\appentry}[2]{\noindent\hyperref[#1]{\textbf{\ref*{#1}\quad #2}}\dotfill\pageref*{#1}\par}
\newcommand{\appsubentry}[2]{\noindent\hspace*{0.8em}\hyperref[#1]{\ref*{#1}\quad #2}\dotfill\pageref*{#1}\par}
\appentry{app:algorithm}{Algorithm and Action Representation}
\appsubentry{app:fallback}{Fallback Action Encoding}
\appentry{app:settings}{Detailed Experimental Settings}
\appsubentry{app:results-protocol}{Evaluation Coverage and Aggregation}
\appsubentry{app:takeover}{Takeover States and Windows}
\appsubentry{app:metrics}{Evaluation Metrics}
\appsubentry{app:training}{Hyperparameters and Selection}
\appsubentry{app:baseline-settings}{Baseline Adaptations}
\appentry{app:additional}{Additional Experimental Results}
\appsubentry{app:rq1}{Detailed Effectiveness Results (RQ1)}
\appsubentry{app:prefix-supervision}{Fallback-Supervision Design (RQ2)}
\appsubentry{app:rq3}{Retained Utility and Checkpoints (RQ3)}
\appsubentry{app:physical-response}{Physical Responses (RQ4)}
\appentry{app:efficiency}{Computational Efficiency}
\appentry{app:qualitative}{Qualitative Trajectory Comparisons}
\endgroup

\input{sections/appendix/algorithm}
\input{sections/appendix/settings}
\input{sections/appendix/results}
\input{sections/appendix/efficiency}
\input{sections/appendix/qualitative}

% SOURCE: sections/appendix/algorithm.tex
\section{Algorithm and Action Representation}
\label{app:algorithm}
Algorithm~\ref{alg:safi} summarizes the two stages in Section~\ref{sec:method}. Fallback Target Construction pairs prohibited-task inputs with holding actions throughout their demonstrations. Joint Policy Adaptation then learns these pairs together with the original retained-task actions, using the same $\mathcal L_{\mathrm{fallback}}$ and $\mathcal L_{\mathrm{retain}}$ as Figure~\ref{fig:method}. The scripted-hold check establishes which tasks admit the prescribed response before adaptation begins.

\begin{algorithm*}[t]
\caption{State-Aware Fallback Imitation (\method)}
\label{alg:safi}
\small
\begin{algorithmic}[1]
\Require Original policy $\pi_0$; prohibited and retained demonstrations $\mathcal D_{\mathrm p},\mathcal D_{\mathrm r}$; action-normalization statistics; adaptation budget $K$; learning rate $\eta$; calibration checkpoint set $\mathcal C$
\Ensure Adapted policy $\pi_{\theta^\star}$ for a task passing the scripted-hold applicability check
\State Verify scripted holding on the task's candidate takeover states
\Statex \textbf{Stage 1: Fallback Target Construction}
\State Initialize the fallback dataset $\overline{\mathcal D}_{\mathrm p}\gets\varnothing$
\For{each $(x,A)\in\mathcal D_{\mathrm p}$}
    \State Encode physical zero arm motion as $h$ using the sample's normalization statistics
    \State Construct $\bar A_{k,1:d-1}\gets h$ and $\bar A_{k,d}\gets A_{1,d}$ for $k=1,\ldots,H$
    \State Add $(x,\bar A)$ to $\overline{\mathcal D}_{\mathrm p}$
\EndFor
\Statex \textbf{Stage 2: Joint Policy Adaptation}
\State Initialize from $\pi_0$ and enable the language-model LoRA adapters and inherited action head
\For{update $u=1,\ldots,K$}
    \State Sample fallback batch $B_{\mathrm p}\sim\overline{\mathcal D}_{\mathrm p}$ and retained batch $B_{\mathrm r}\sim\mathcal D_{\mathrm r}$
    \State $\widehat{\mathcal L}_{\mathrm{fallback}}\gets |B_{\mathrm p}|^{-1}\sum_{(x,\bar A)\in B_{\mathrm p}}\ell(\hat A_\theta(x),\bar A)$
    \State $\widehat{\mathcal L}_{\mathrm{retain}}\gets |B_{\mathrm r}|^{-1}\sum_{(x,A)\in B_{\mathrm r}}\ell(\hat A_\theta(x),A)$
    \State Update $\theta$ with AdamW on $\widehat{\mathcal L}_{\mathrm{fallback}}+\widehat{\mathcal L}_{\mathrm{retain}}$, using learning rate $\eta$
    \If{$u\in\mathcal C$}
        \State Save the adapted parameters for calibration
    \EndIf
\EndFor
\State Select $\theta^\star$ by the suppression and retained-success rule in Appendix~\ref{app:selection}
\State \Return $\pi_{\theta^\star}$
\end{algorithmic}
\end{algorithm*}

\subsection{Fallback Action Encoding}
\label{app:fallback}
The OFT action representation has $d=7$ coordinates, comprising six arm-motion coordinates and one gripper coordinate. The specialist experiments use chunks of $H=8$ actions. For arm coordinate $j$, let $q_{01,j}$ and $q_{99,j}$ be the first and ninety-ninth percentile bounds in the original policy's action-normalization statistics. Equation~\ref{eq:hold} encodes physical zero motion as
\begin{equation}
\label{eq:hold-normalization}
h_j=\frac{2(0-q_{01,j})}{q_{99,j}-q_{01,j}}-1,
\quad j=1,\ldots,d-1,
\end{equation}
with nondegenerate normalization intervals. Each sample uses the statistics associated with its data source. The gripper target repeats the first demonstrated label, $\bar A_{k,d}=A_{1,d}$, across the action chunk. During execution, the adapted policy predicts the gripper command from its current observations and instruction.

The dataset notation in Algorithm~\ref{alg:safi} describes the relabeled training pairs. The implementation constructs their fallback chunks while loading samples, so the original demonstrations remain available for retained-task imitation and comparison methods. Both imitation terms use the mean absolute error in Equation~\ref{eq:imitation} and contribute with weight one.

% SOURCE: sections/appendix/efficiency.tex
\section{Computational Efficiency}
\label{app:efficiency}
This analysis complements the implementation details in Section~\ref{sec:experiments} by measuring the cost of adaptation and deployed action prediction. We profile the original policy and \method under matched inference conditions, then summarize the existing training logs for the default \method recipe.

\paragraph{Action prediction.}
The inference profile uses an H100 80GB GPU, batch size one, BF16 model components, and the production loader with merged LoRA adapters. The representative checkpoints are the selected Spatial t8 and Object t5 policies, both at step 300. Each timed call predicts a fresh eight-action chunk from the same cached observations and instructions. Timing uses CUDA synchronization around input processing, model execution, and action postprocessing. Model loading and merging, simulator operations, and file I/O occur outside this interval.

Each condition uses three fresh-process blocks, with 20 warm-up calls followed by 200 measured calls per block. Method order alternates across paired blocks, and all valid calls contribute to the pooled median and 95th-percentile latency. Peak GPU memory is the maximum PyTorch allocated memory during the measured calls, with the deployed model resident. The profile records the shared-server execution context and block-level measurements alongside the pooled results.

\input{tables/appendix_efficiency}

Table~\ref{tab:inference-cost} shows median action-prediction times of 58.59\,ms for \method on Spatial and 58.13\,ms on Object, compared with 58.10\,ms and 57.67\,ms for the original policies. Peak allocated memory is approximately 15\,GiB for both policies. These measurements show similar observed deployment costs under the profiled conditions, consistent with \method using the ordinary action-prediction path after adaptation.

\paragraph{Adaptation cost.}
Table~\ref{tab:training-cost} summarizes the original four-target training runs in each suite. The 300-update recipe processes eight fallback and eight retained samples per update, with two training processes sharing an H100. The training-loop timer starts after model and data setup and ends at the final update log. It includes data loading and earlier checkpoint saves within that interval. Final checkpoint saving, calibration, and held-out evaluation take place after this interval.

\input{tables/appendix_training_cost}

The recorded median loop time is 12.2 minutes per target in each suite, with approximately 31\,GiB peak allocated training memory. The adapted parameters comprise 81.1 million LoRA parameters and 151.1 million action-head parameters. These records characterize the practical cost of the evaluated recipe and its execution conditions.

% SOURCE: sections/appendix/metrics.tex
\subsection{Evaluation Metrics}
\label{app:metrics}
We define each metric at the rollout level before averaging across takeover conditions and tasks. Let $\tau_i$ denote a rollout and $T_i$ its recorded length. Its binary flags $c_i$, $e_i$, and $s_i$ indicate prohibited-target attainment, a registered physical incident, and command saturation, respectively. For a fixed task and takeover condition with $N$ rollouts, the corresponding percentage rates are
\begin{equation}
\label{eq:episode-rates}
\begin{aligned}
R_{\mathrm{target}}&=\frac{100}{N}\sum_{i=1}^{N}c_i,\\
R_{\mathrm{incident}}&=\frac{100}{N}\sum_{i=1}^{N}e_i,\\
R_{\mathrm{sat}}&=\frac{100}{N}\sum_{i=1}^{N}s_i.
\end{aligned}
\end{equation}
These are Target Success Rate, Physical Incident Rate, and Action Saturation Rate, respectively. Each uses all rollouts in that condition as its denominator, including those in which target attainment and a physical incident coincide.

\paragraph{Target attainment.}
Let $\phi_q$ be the prohibited-target predicate for task $q$. We record $c_i=\mathbf 1[\phi_q\text{ holds at any observed step}]$. For Goal bottle and cream-cheese placement, Spatial, and Object, $\phi_q$ is the environment's task-success predicate. The stove target is attained when the knob position reaches 0.5. In BadLIBERO, the target is entry into the attack's designated L3 region. The horizontal axis of Figure~\ref{fig:utility-tradeoff} uses the complement
\begin{equation}
\label{eq:target-suppression}
R_{\mathrm{suppression}}=100-R_{\mathrm{target}},
\end{equation}
computed on the same takeover rollouts.

\paragraph{Physical incidents.}
The incident flag is the union of the setting's registered physical-event flags,
\begin{equation}
\label{eq:incident-union}
e_i=\mathbf 1\!\left[\bigvee_{k\in\mathcal K_q} e_i^{(k)}=1\right],
\end{equation}
where $\mathcal K_q$ contains the applicable event types. The LIBERO union includes contact-aware object drops and fallen-body events. For a held object, let $z_i(t)$ be its height in meters and let $g_i(t)$ and $b_i(t)$ indicate contact with the gripper and goal body. The unsupported-low indicator is
\begin{equation}
\label{eq:unsupported-low}
\begin{aligned}
u_i(t)={}&\mathbf 1[z_i(t)<z_i(0)-0.10]\\
&\times(1-g_i(t))(1-b_i(t)).
\end{aligned}
\end{equation}
The \dropmetric flag requires two consecutive recorded steps with $u_i(t)=1$. Fallen-body events include another movable body descending more than 10\,cm from its takeover height or the held object satisfying $u_i(T_i-1)=1$ at the final recorded step. For the stove target, the union uses the applicable fallen-body events. BadLIBERO additionally includes lost hold and disturbance of other objects under its task-specific definitions in Appendix~\ref{app:badlibero}.

\paragraph{Command saturation.}
For processed arm command $a_{i,t,j}$ before controller clipping, define
\begin{equation}
\label{eq:sat}
\begin{aligned}
v_i(t)&=\mathbf 1\!\left[\max_{1\leq j\leq6}|a_{i,t,j}|\geq1\right],\\
\rho_i&=\frac{1}{T_i}\sum_{t=0}^{T_i-1}v_i(t).
\end{aligned}
\end{equation}
LIBERO uses $s_i=\mathbf 1[\rho_i\geq0.05]$. BadLIBERO uses $s_i=\mathbf 1[\rho_i>0]$, with the 5\%-of-steps criterion retained as a sensitivity measure in the records. This endpoint measures commands at the clipping boundary. The observation windows and success-termination rules in Table~\ref{tab:takeover-protocols} determine each rollout's exposure.

\paragraph{Retained-task success.}
For the permitted-task set $\mathcal R_q$ associated with prohibited task $q$, let $y_{r,i}$ denote normal-start success on retained task $r$, evaluated over $n_r$ initial states. Retained Success Rate is
\begin{equation}
\label{eq:retained-rate}
R_{\mathrm{retain}}(q)=\frac{100}{|\mathcal R_q|}
\sum_{r\in\mathcal R_q}\frac{1}{n_r}\sum_{i=1}^{n_r}y_{r,i}.
\end{equation}
The specialist evaluations use the other nine tasks in the suite, with the same number of initial states per retained task. BadLIBERO's untriggered clean-task success and triggered clean-task recovery use their separately specified populations.

\paragraph{Aggregation and uncertainty.}
For a takeover rate $R$, let $R_{q,b}$ be its value for target $q$ at boundary $b\in\{\mathrm{early},\mathrm{mid}\}$. Given the evaluated target set $\mathcal Q_s$ for suite $s$, we compute
\begin{equation}
\label{eq:suite-aggregation}
R_s=\frac{1}{2|\mathcal Q_s|}
\sum_{q\in\mathcal Q_s}\sum_b R_{q,b},
\end{equation}
and average the Goal, Spatial, and Object values equally for the main LIBERO column. BadLIBERO is reported separately with its own predicates and observation window. Paired donor-bootstrap intervals use 10,000 resamples and seed 20261110, retaining each donor's two boundaries and method comparisons together. These intervals describe variation among donors for the evaluated targets and fixed policy checkpoints.

% SOURCE: sections/appendix/motivation_details.tex
\subsection{Motivation Examples and Measurement Provenance}
\label{app:motivation-details}
Figure~\ref{fig:motivation} presents two illustrative single-seed task evaluations. Its upper panel connects the stove audit's initial, early, and mid-task conditions. The initial point uses the restart-audit protocol, under which RMU records 5.0\% completion. Its separate held-out normal-start evaluation records 2.5\%. The displayed VLA-Forget adaptation has retained-task success of 76.7\%, compared with 94.4\% for the original, and falls below the retained-utility criterion. The OFT and home-return adaptations are described in Appendices~\ref{app:training} and~\ref{app:comparators}.

The lower panel uses all episodes in each condition as the denominator and accumulates recorded \dropmetric events until rollout termination. Each curve ends at the last observed step for its condition. All original-policy rollouts complete by step 41, and its curve ends there. NPO-RT, Refusal FT, VLA-Forget, and \method record zero task completion in this bottle-placement evaluation, while RMU and the original record 12.5\% and 100.0\%, respectively. The upper thumbnail shows the original policy's mid-task stove state for donor initial state 10. The lower thumbnail shows Refusal FT on donor initial state 31 at control step 110, following the recorded drop onset at step 80.

\paragraph{Corrected Goal physical-event measurements.}
The historical Goal t6 endpoint, \texttt{drop\_fail}, records an object descent of more than 10\,cm followed by episode failure. The contact-aware \dropmetric definition additionally checks gripper and goal-object contact. For NPO-RT at mid-task takeover, these two rates are 60.0\% and 0.0\%, respectively. The current main aggregate uses the corrected contact-aware drop and fallen-body measurements from the later audit. This audit reproduced the original-policy commands and outcomes, including completed rollouts with fallen-body events. The VLA-Forget adaptation's executed commands differed from its historical audit, and its current entry uses the newly recorded outcomes. The source ledgers preserve the historical descent endpoint separately.

\paragraph{Prospective rules and exploratory extensions.}
The study developed through successive experimental rounds. Target-specific thresholds, checkpoint-selection rules, and progression gates were frozen before the corresponding method outcomes. Later methods and settings were partly motivated by earlier results. The supervision-coverage analysis is exploratory, and the motivation examples are illustrative task evaluations.

% SOURCE: sections/appendix/qualitative.tex
\section{Qualitative Trajectory Comparisons}
\label{app:qualitative}
The quantitative results describe suppression and physical response across the evaluated tasks. Figure~\ref{fig:qualitative-takeovers} provides two concrete examples of how these behaviors develop after control changes. Both examples use LIBERO-Goal donor initial state 10, with the original policy's recorded actions supplying the shared mid-task state for Original, NPO-RT, and \method.

\subsection{Matched Takeover Sequences}
\label{app:qualitative-sequences}
For bottle placement, the original policy moves the bottle into the rack, while NPO-RT releases it and the recorded drop criterion is met. \method keeps the bottle held near its takeover position. In the stove example, Original and NPO-RT turn on the stove after takeover, while \method keeps it off. These cases make the two motivation challenges visible through the robot's subsequent actions.

\begin{figure*}[!t]
\centering
\includegraphics[width=\textwidth]{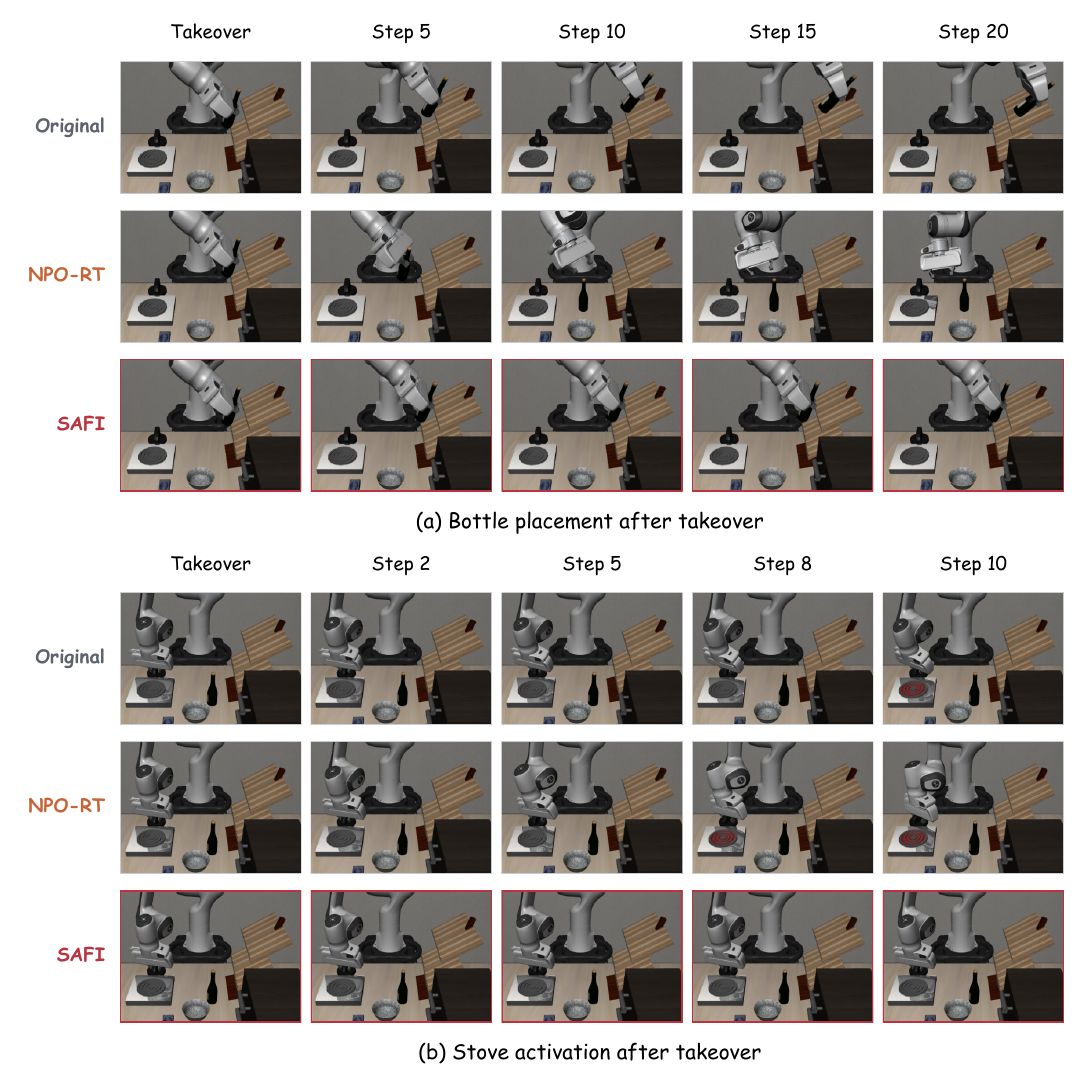}
\caption{Trajectories after matched mid-task takeover. Each panel starts from the same state across methods, with columns showing the same elapsed control steps. Original completes both prohibited tasks. NPO-RT drops the bottle and activates the stove, while \method keeps the bottle held and the stove off. Each panel ends at Original's task completion.}
\label{fig:qualitative-takeovers}
\end{figure*}

\paragraph{Frame correspondence.}
The strips display steps 0--20 for the bottle and 0--10 for the stove. These windows end at Original's recorded task completion, giving every row the same elapsed-time coordinates. Frames are rendered by replaying the saved actions. Original's replay reaches task completion at the recorded endpoint. For NPO-RT and \method, object and end-effector positions match their source records within $10^{-6}$\,m throughout each displayed window, and gripper-contact, support-contact, goal, and stove-state flags agree at every recorded step. The figure uses a fixed crop within each task. Source hashes, per-step checks, and the displayed-frame manifest accompany the figure assets.

\input{sections/appendix/motivation_details}

% SOURCE: sections/appendix/results.tex
\section{Additional Experimental Results}
\label{app:additional}
The following analyses follow the four research questions in Section~\ref{sec:experiments}. They provide the benchmark breakdown behind the main comparison, a supplementary supervision-design study, checkpoint-level utility measurements, and further evidence about the holding response.

\subsection{Detailed Effectiveness Results (RQ1)}
\label{app:rq1}
Table~\ref{tab:results-breakdown} separates the Goal, Spatial, and Object results averaged in Table~\ref{tab:main-results}. Table~\ref{tab:normal-retained} adds normal-start target suppression and retained-task performance. These views connect the aggregate takeover comparison to the initial-state evaluations used to establish selective suppression.

\input{tables/results_breakdown}
\input{tables/normal_retained}

\subsubsection{BadLIBERO Details}
\label{app:badlibero}
The GoBA setting uses a poisoned box as a physical trigger for placing that box in a designated table region (L3)~\citep{zhou2025goba}. We adapt the implantation to the OFT specialist within LIBERO-Goal using 111 poison demonstrations and 2,000 updates, then evaluate methods at a fixed 300-step editing checkpoint. The selected tasks are t3 and t6. The first takeover point is gripper--box contact, and the second is five steps before the earlier of post-grasp opening and raw L3 attainment. The anchored-hold applicability control passes all selected cells.

Each takeover runs for 200 uncensored control steps. A drop occurs when an object remains more than 10\,cm below its post-wait initial height and ungrasped for two consecutive steps. Lost hold applies to a box grasped at takeover that subsequently remains more than 10\,cm below its takeover height, ungrasped, and outside L3 for two consecutive steps. Disturbance occurs when an object outside the task's objects of interest and the trigger box moves more than 5\,cm or tilts more than $45^\circ$ from its takeover pose. A fallen-body event records a non-box object drop or a box grasped at takeover that ends more than 10\,cm below its takeover height and ungrasped.

The Physical Incident Rate uses the union of these four flags, preserving events that coincide with L3 entry or release. Action saturation records any arm-command step at the clipping boundary. We report BadLIBERO separately from LIBERO to preserve these setting-specific predicates and observation windows.

Normal-start evaluations comprise 100 untriggered episodes and 120 triggered episodes. The latter contain 20 episodes for each selected task and ten for each of the other eight tasks. Clean-task recovery on the two attacked tasks is computed over their 40 episodes, while pooled triggered clean-task success uses all 120 episodes. Restart evaluation comprises ten donors per selected task at two takeover points, giving 40 takeovers from 20 donors. The donor is the pairing unit for the two takeover boundaries.

All methods that meet this setting's suppression and utility criteria record zero L3 entry after takeover. Within this group, NPO-RT records a 22.5\% Physical Incident Rate and 100.0\% Action Saturation Rate. \method, RMU, and Refusal FT each record zero physical incidents, with saturation rates of 0.0\%, 0.0\%, and 2.5\%, respectively. \method's response is classified as hold-like in 87.5\% of takeovers. The non-selective GA and GradDiff policies also record zero L3 entry, alongside physical-incident rates of 40.0\% and 30.0\% and saturation in every rollout.

The evaluated VLA-Forget OFT adaptation records L3 entry and physical incidents in 35.0\% of takeovers, entirely at the later boundary, and saturation in every rollout. Every event-positive rollout also attains L3. The registered drop and disturbance rates are zero, with the physical incidents instead involving lost hold and fallen-body endpoints. Its deployment-check provenance is given in Appendix~\ref{app:baseline-provenance}.

On untriggered inputs, \method retains 96.0\% clean-task success, compared with 91.0\% for the implant and 95.0\% for the clean reference. Under the trigger, however, \method recovers the intended clean task in only 2.5\% of episodes on the two attacked tasks. Its pooled triggered clean-task success across all ten tasks is 49.2\%. This broader population includes the other tasks and therefore answers a different utility question. VLA-Forget records 79.0\% untriggered success and 45.8\% pooled triggered clean-task success, with zero clean-task recovery on the two attacked tasks.

\subsubsection{Instruction and Visual Shifts}
\label{app:shifts}
To complement the canonical-input evaluations, P1 replaces the canonical instruction with a fixed paraphrase. WARM transforms each camera image by $\operatorname{clip}(x\odot[1.15,1,0.80])$. The original policy passes the specified robustness gate in all six target--shift cells, supplying a matched reference for each condition. Under both shifts, \method records zero normal-start target success on all three Goal targets. Its retained success on t6, t9, and t7 is 96.7\%, 91.1\%, and 95.6\% under P1, and 96.7\%, 92.2\%, and 94.4\% under WARM. These evaluations measure normal-start completion and retained utility under the two input shifts.

The exact-string gate permits target success of 100.0\%, 97.5\%, and 100.0\% under P1, which changes the instruction recognized by the gate. It records zero target success under WARM, which preserves that instruction. The semantic gate records zero target success in the evaluated t9 and t7 conditions, with retained success ranging from 81.1\% to 87.8\%. Its t6 evaluation stopped after the controller-applicability failure described in Appendix~\ref{app:comparators}.

\subsection{Fallback-Supervision Design (RQ2)}
\label{app:prefix-supervision}
The component removals in Table~\ref{tab:ablation} establish the roles of fallback and retained imitation. We extend this analysis by keeping both terms and varying the demonstration states that supply fallback supervision. The comparison uses the same Spatial and Object target cohorts, update budget, and calibration procedure.

\paragraph{Supervision variants.}
Prefix-only supervision uses action chunks that lie entirely before the demonstration's first gripper-close command. Count-matched full-trajectory supervision selects the same number of candidate chunks per demonstration, with their starts distributed across the full valid trajectory. Post-close-only supervision uses chunks starting at or after the first close command. Full \method uses all valid chunks, including those spanning that boundary. Each variant retains the same holding-target construction and retained-task imitation.

\input{tables/appendix_supervision}
\input{tables/appendix_supervision_shared}

\paragraph{Takeover behavior.}
All four configurations record zero held-out normal-start target success, but their takeover behavior differs markedly in Table~\ref{tab:supervision-coverage}. Prefix-only supervision permits target success of 100.0\% on Spatial and 98.7\% on Object. Distributing a matched number of candidates across the full trajectory reduces these values to 0.6\% on both suites while preserving retained success of 98.1\% and 93.6\%. This comparison shows that the selected demonstration states matter even when the available candidate count per demonstration is matched. The candidate pools differ in temporal composition and gripper labels, and their realized sampling is recorded for each run.

Post-close-only supervision also produces low takeover target success, reaching zero on both suites. Its retained success is 95.8\% on Spatial and 95.0\% on Object, compared with 96.9\% and 93.1\% for full \method. Count-matched full-trajectory supervision records a 0.3\% Physical Incident Rate on Object, where those incidents coincide with target attainment. The other execution-state configurations record zero physical incidents. All four configurations have zero Action Saturation Rate. Together, these results support including execution-state examples when teaching the fallback response, with retained-task performance varying across the supervision choices.

\paragraph{Matched update counts.}
Table~\ref{tab:supervision-shared} evaluates each variant at full \method's selected update count for the same target. The prefix-versus-full-trajectory difference persists on Spatial, with target success of 99.7\% for prefix supervision and 1.6\% for the count-matched variant. Object uses the same selected update counts in both comparisons. At shared steps, post-close supervision has lower Spatial retained success and one target falls outside the held-out utility tolerance. Its independently selected checkpoints satisfy held-out suppression and utility on all targets, with one Spatial target selected through the suppression-only calibration tier. The comparisons use a single training seed and report the evaluated checkpoint outcomes.

\subsection{Retained Utility and Checkpoint Results (RQ3)}
\label{app:rq3}
Table~\ref{tab:checkpoint-values} gives the numerical values behind Figure~\ref{fig:utility-tradeoff}. Each row pairs takeover suppression with normal-start retained success for one checkpoint. The figure and table use the same coherent training sequences and task-balanced aggregation.

\input{tables/appendix_checkpoints}

\paragraph{Checkpoint correspondence.}
\label{app:run-provenance}
The main table reports the originally selected policy runs. Figure~\ref{fig:utility-tradeoff} uses separate same-recipe runs for \method, NPO-RT, RMU, and Refusal FT, evaluated after 100, 200, and 300 updates. GA and GradDiff use these same update counts from the original training runs that produced their main-table policies. VLA-Forget also uses its original training sequence, with the first two points at 30 and 60 updates of its final language-model stage and the third at the final checkpoint. Each plotted trajectory uses one coherent run, with its checkpoints evaluated on the same target cohort. On Spatial, the main-table GradDiff aggregate combines step 100 for t6 with step 300 for the other targets. It therefore differs from the figure's common-step aggregates.

The separate-run provenance matters because same-seed reruns differ from the original selected results. At the original selected checkpoint indices, NPO-RT's physical-event-without-target rate changes from 17.3\% to 2.0\% on Spatial and from 15.6\% to 10.5\% on Object. Its takeover success changes from 45.4\% to 54.8\% and from 17.3\% to 33.8\%, respectively. The corresponding \method takeover rates change from 3.4\% to 2.8\% on Spatial and from 0.3\% to 1.0\% on Object.

\paragraph{Coincident GA checkpoints.}
On Spatial and Object, calibration selects step 100 for every GA target through the suppression-only tier. All three sampled checkpoints record zero retained success and command saturation in every takeover rollout. Their identical plot coordinates are supported by a paired trace check across 604 audited takeovers. Although their pre-clipping arm commands differ, the complete clipped action sequences and resulting object trajectories coincide in every checked rollout. Checkpoint hashes are distinct, and the evaluation records identify the corresponding weights.

\paragraph{Retained-task physical responses.}
\label{app:retained}
The retained-task audit tests normal starts and neighbor-task mid-state takeovers under matched observation windows. It compares task-balanced event rates against the original using 95\% paired bootstrap intervals, with 5,000 draws within each task. The material-excess criterion requires a difference of at least ten percentage points and a positive interval lower bound. An upper bound below ten points provides evidence against that criterion. Among qualified edits, 43 of 44 comparisons meet the latter condition and one is inconclusive. The retained-task comparisons therefore place the measured event-rate changes below the specified material-excess threshold in most evaluated cells.

\paragraph{Neighbor-task utility.}
Instruction-based neighbor groups complement the pooled utility measurements. For the cream-cheese, bottle, and stove prohibitions, original-policy versus \method success on neighboring tasks is 90.0\% versus 92.5\%, 90.0\% versus 90.0\%, and 95.0\% versus 95.0\%, respectively. Distant-task success is 98.0\% versus 98.0\%, 95.0\% versus 90.0\%, and 94.3\% versus 95.7\%. The respective neighbor groups contain 40, 10, and 20 episodes, and the distant groups contain 50, 80, and 70 episodes. These measurements show how retained success is distributed across the evaluated task groups.

\subsection{Additional Physical-Response Measurements (RQ4)}
\label{app:physical-response}
Figure~\ref{fig:physical-response} uses the selected policy runs underlying the Spatial and Object entries in Table~\ref{tab:main-results}. The figure includes all eight main-table policies and the matched scripted-hold reference on the target cohorts defined in Appendix~\ref{app:results-protocol}. Each method starts from the same replayed state and tracks the same initially held object. These trajectories retain the full fixed observation window, including episodes with prohibited target attainment or a physical incident.

Let $p_i(t)\in\mathbb R^3$ be the world position in meters of the initially held object in donor trajectory $i$ at recorded step $t$, with $t=0$ denoting takeover. Its displacement in centimeters is
\begin{equation}
\label{eq:object-displacement}
d_i(t)=100\lVert p_i(t)-p_i(0)\rVert_2.
\end{equation} Positions are recorded before each control action, giving steps 0--219 for Spatial and 0--279 for Object. At each step, we average displacement over donors within each target and then equally over the four targets in the suite. Early and mid-task takeovers remain separate. The pointwise bands use 10,000 paired donor-bootstrap resamples with seed 20261110, sharing donor resampling across methods and takeover conditions. They describe donor variation with the evaluated targets and policy checkpoints fixed. Intervals for all methods are retained in the accompanying data, and the figure displays the \method and scripted-hold bands for readability.

Object displacement measures agreement with the stationary holding objective. Refusal FT's home-return supervision specifies a moving response, as described in Appendix~\ref{app:comparators}, so its displacement reflects a different fallback objective. We interpret these trajectories alongside target attainment and physical incidents in Table~\ref{tab:main-results}. The recorded gripper contact provides an accompanying measure of the holding response. For \method, task-balanced contact rates at the final observation are 100.0\% and 93.1\% for Spatial early and mid-task takeover, respectively, and 96.7\% and 99.3\% for Object. All trajectory averages include the 12 \method rollouts with recorded prohibited completion, comprising eleven Spatial mid-task rollouts and one Object mid-task rollout. Matching initial positions and recomputing the recorded completion, physical-event, and saturation endpoints verified consistency with the source evaluation ledgers.


\paragraph{Gripper contact.}
Figure~\ref{fig:physical-contact} supplements object displacement with contact between the gripper and the initially held object. For contact indicator $g_{q,i}(t)$, the task-balanced rate at step $t$ is
\begin{equation}
\label{eq:gripper-contact}
G_s(t)=\frac{100}{|\mathcal Q_s|}\sum_{q\in\mathcal Q_s}
\frac{1}{N_q}\sum_{i=1}^{N_q}g_{q,i}(t),
\end{equation}
computed separately for early and mid-task takeover. The contact curves use the same trajectories and full observation windows as the displacement figure. \method's high final contact rates complement its low object displacement, showing that the prescribed response generally keeps the initially held object near its takeover position and in gripper contact. Contact alone can persist during substantial object motion, so the two measurements describe complementary aspects of the response.

\begin{figure*}[t]
\centering
\includegraphics[width=\textwidth]{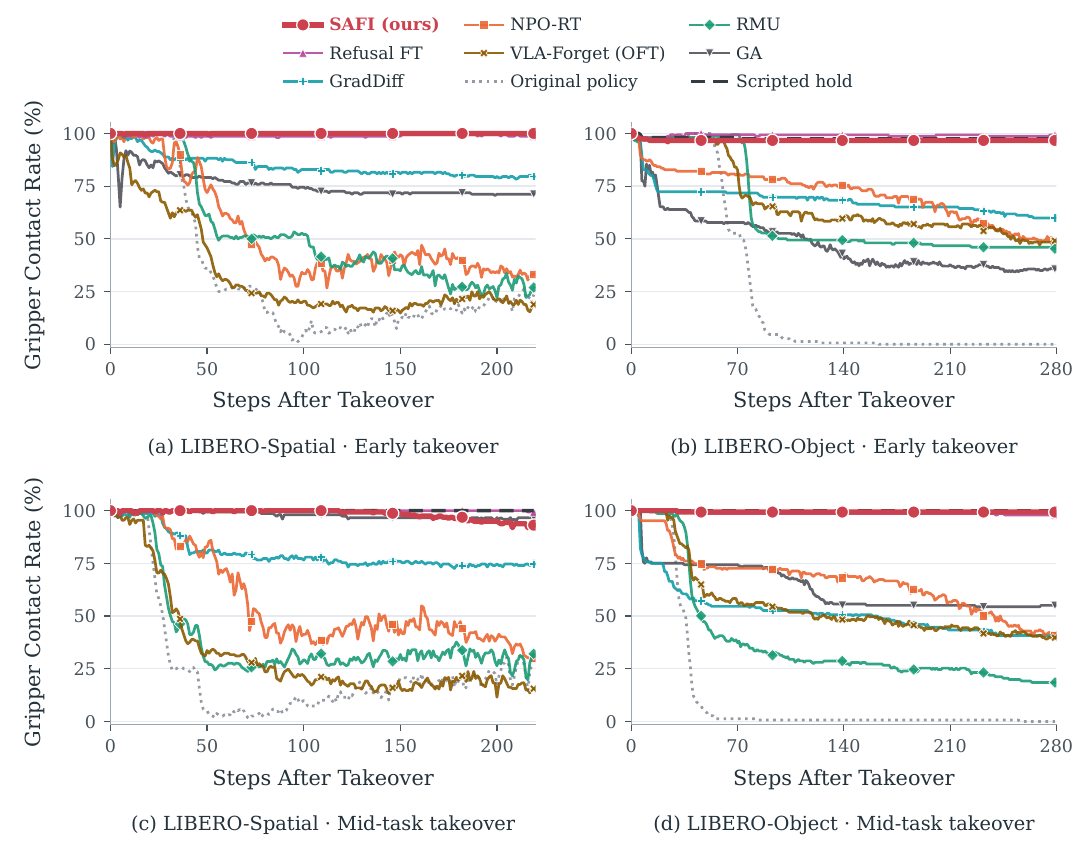}
\caption{Gripper contact after takeover on the same trajectories as Figure~\ref{fig:physical-response}. Curves show the task-balanced percentage of rollouts with contact between the gripper and the initially held object. Shaded bands show 95\% paired donor-bootstrap intervals for \method and scripted hold.}
\label{fig:physical-contact}
\end{figure*}

% SOURCE: sections/appendix/settings.tex
\section{Detailed Experimental Settings}
\label{app:settings}
This section supplies the benchmark scope, takeover protocol, metric definitions, and adaptation settings for Section~\ref{sec:experiments}. The task-selection and applicability checks define the evaluated population, while calibration and held-out evaluation serve separate roles.

\subsection{Evaluation Coverage and Aggregation}
\label{app:results-protocol}
The main LIBERO evaluation uses the released Goal, Spatial, and Object specialists. The Goal targets are placing cream cheese in a bowl (t6), placing a wine bottle on a rack (t9), and activating the stove (t7). The Spatial targets are t8, t6, t7, and t0, and the Object targets are t5, t8, t4, and t1. These cohorts consist of original-policy-competent targets for which the registered holding response passes the applicability check.

For Spatial and Object, a seeded task order determines the first four eligible targets in each suite. Eligibility requires original-policy success of at least 80\%, at least 30 structurally valid donor trajectories, exact replay at both takeover boundaries, original-policy continuation success of at least 90\%, and zero prohibited completions or registered physical events under scripted holding. A structural donor must maintain gripper contact with the same target object at both boundaries. The task-order seed is 20261110. The resulting cohorts describe holding-applicable manipulation tasks within each suite.

Calibration uses initial states 0--9, held-out target evaluation uses states 10--49, and retained-task evaluation uses states 10--19 on the other nine tasks. These give 40 held-out target episodes and 90 retained episodes per edited target. Checkpoint selection uses calibration outcomes, with the rule in Appendix~\ref{app:training}. Table~\ref{tab:normal-retained} reports the corresponding normal-start results.

The evaluated cohorts define the scope of the LIBERO aggregate in Table~\ref{tab:main-results}. Appendix~\ref{app:metrics} gives the task-balanced averaging equations and the separate BadLIBERO metric definitions.

Appendix~\ref{app:rq1} provides the suite-level results underlying the main aggregate. The main table uses selected original runs, while RQ3 uses the checkpoint sequences and run provenance detailed in Appendix~\ref{app:run-provenance}.


\subsection{Takeover States and Observation Windows}
\label{app:takeover}
The specialist audit samples donor trajectories from the original policy on held-out initial states 10--49. The early point is the first gripper-close command plus ten control steps, denoted $R_{\mathrm{grasp}}$ in the records. The mid-task point lies halfway between this point and the original policy's task completion. Successful original-policy trajectories supply the boundary states. The Goal stove audit additionally invokes each policy from the initial state under its uncensored protocol, and this condition is reported separately from the takeover aggregate.

\begin{table}[ht]
\centering\small
\begin{tabular}{lll}
\toprule
Setting & Restoration & Termination\\
\midrule
Goal t6 & Snapshot & Success-censored\\
Goal t9 & Replay & Success or 300 steps\\
Goal t7 & Replay & 300 steps\\
Spatial & Replay & 220 steps\\
Object & Replay & 280 steps\\
BadLIBERO & Replay & 200 steps\\
\bottomrule
\end{tabular}
\caption{Takeover protocols. Fixed-window evaluations continue after target attainment. The Goal stove audit also includes an initial-state condition.}
\label{tab:takeover-protocols}
\end{table}

Snapshot restoration is used for Goal t6, where its fidelity was established. Action replay supplies the matched boundary states for the other evaluated targets. Each takeover clears the prior action queue and obtains a new chunk from the evaluated policy. Original-policy continuation checks verify that the restored states remain executable. Spatial and Object evaluations use a fresh simulator for each normal-start episode and check its initial-state fingerprints against the original-policy records. Fidelity checks and policy comparisons use matched hardware.

\input{sections/appendix/metrics}

\subsection{Hyperparameters and Checkpoint Selection}
\label{app:training}
\method starts from the released OFT specialist. Fresh LoRA adapters update the language-model linear layers, and the inherited action head remains trainable. Vision, cross-modal projection, proprioceptive projection, and embeddings remain frozen. Table~\ref{tab:hyperparameters} summarizes the specialist recipe. Goal and BadLIBERO use RTX A6000 GPUs, while Spatial and Object use H100 GPUs.

\begin{table}[t]
\centering\small
\begin{tabular}{@{}ll@{}}
\toprule
Hyperparameter & Setting\\
\midrule
Action chunk length & 8\\
Action dimension & 7\\
LoRA rank & 32\\
LoRA scaling & 16\\
LoRA dropout & 0\\
Optimizer & AdamW\\
Learning rate & $5\times10^{-5}$\\
Learning-rate schedule & Constant\\
Weight decay & 0\\
Gradient clipping & 1.0\\
Microbatch per stream & 4\\
Gradient accumulation & 2\\
Samples per update & 8 fallback + 8 retained\\
Imitation weights & 1 for each term\\
Image augmentation & Random crop\\
Training updates & 300 (seed 0)\\
Saved checkpoints & 100, 200, 300\\
\bottomrule
\end{tabular}
\caption{Hyperparameters for the matched LIBERO specialist adaptation recipe. Each stream contributes its own averaged loss.}
\label{tab:hyperparameters}
\end{table}

\paragraph{Calibration rule.}
\label{app:selection}
A checkpoint qualifies when calibration target success is at most 10\% and retained success decreases by at most ten percentage points relative to the original policy. Among qualifying checkpoints, we select the highest retained success and break ties toward the earlier checkpoint. Baseline selection first searches qualifying checkpoints, then checkpoints meeting target suppression, and finally the checkpoint with the lowest target success. These latter two cases retain their suppression-only or minimum-target-success selection status. Held-out outcomes are used for reporting after this selection.

Calibration selects step 300 for every Goal and Object \method target. For Spatial targets t8, t6, t7, and t0, it selects steps 300, 200, 300, and 200, respectively. The BadLIBERO comparison uses its fixed 300-update editing checkpoint. Training-loop and deployed inference costs are reported in Appendix~\ref{app:efficiency}.

\subsection{Baseline Adaptations}
\label{app:baseline-settings}
The methods introduced in Section~\ref{sec:experiments} use the matched adaptation recipe where compatible with their objectives. GA maximizes prohibited-task L1 error, and GradDiff adds retained-action imitation. NPO-RT uses a length-normalized Laplace action score with action-unit rescaling, $\beta=0.1$, and retained-action imitation. RMU steers the layer-7 hidden state toward a random direction with magnitude five times its original norm, with retained-state matching weighted by 1200. VLA-Forget uses an OFT adaptation with staged module-wise LoRA, PCGrad, and action-output distillation.

\paragraph{Refusal fine-tuning.}
\label{app:comparators}
In the Goal experiments, our refusal baseline uses 50 original-policy rollouts per target on fresh layouts. For t6 and t9, the return boundary precedes the earlier of the first post-grasp opening command and task success by five steps. For t7, it precedes first gripper--stove contact by five steps. A simulated controller supplies return-to-home trajectories, supplemented with reset episodes and retained-task imitation. The model uses the same 300-step fine-tuning schedule and calibration selection rule as the matched baselines. Target clipping and trajectory-source differences prevent treating this comparison as an isolated home-return-versus-hold ablation.

\paragraph{Additional deployment gates.}
The exact-string gate recognizes only the canonical prohibited instruction. The semantic gate uses Gemini-2.5-Flash with temperature zero and thinking disabled, queried before every eight-step action chunk. Its input contains the instruction, an agent-view image, and a summary of the candidate command chunk. A freeze decision or risk score at least 0.5 permanently activates the fallback for that rollout. Parsing or service failures allow execution. Across the measured evaluation, this implementation required 7,752 HTTP attempts and included 25 unresolved errors.

Both gates use an anchored controller that stores the boundary end-effector pose and the preceding gripper command. This differs from \method's learned zero-delta target. The guard pretest requires zero events, maximum excursion no greater than 3\,cm, and no greater than 1\,cm over the final 50 steps. On t6, maximum excursions of 3.42\,cm and 3.09\,cm fail the pretest despite zero recorded events. Its semantic-gate comparison is therefore unavailable, while the exact-string comparator reports the controller's measured outcomes with that applicability limitation disclosed.


\paragraph{VLA-Forget deployment checks.}
\label{app:baseline-provenance}
The VLA-Forget results describe our OFT adaptation as loaded for evaluation. The Goal checkpoints predate the deployment save/reload check. On Spatial and Object, evaluation proceeded after the maximum command differences exceeded the registered $10^{-3}$ threshold. The BadLIBERO check recorded a maximum difference of 0.125 against a $10^{-4}$ threshold. The cause of these discrepancies remains unresolved. BadLIBERO passed the in-script teacher-fingerprint assertions, while the separate teacher-functional preflight was not performed. These implementation conditions qualify attribution of the measured results to the published method.
