# Supplementary material for: Teaching Vision-Language-Action Models to Stop Safely
Source: arXiv:2611.26239 source file (2026-11-19)
Supplement: Supplementary file 2 [file appendix_before_restructure_20261117.tex]

\section{Audit Protocols and Detailed Results}
\label{app:protocol}
\subsection{Evaluation Coverage and Aggregation}
\label{app:results-protocol}
The main LIBERO evaluation uses the released Goal, Spatial, and Object specialists. The Goal targets are placing cream cheese in a bowl (t6), placing a wine bottle on a rack (t9), and activating the stove (t7). The Spatial targets are t8, t6, t7, and t0, and the Object targets are t5, t8, t4, and t1. These cohorts consist of original-policy-competent targets for which the registered holding response passes the applicability check.

For Spatial and Object, a seeded task order determines the first four eligible targets in each suite. Eligibility requires original-policy success of at least 80\%, at least 30 structurally valid donor trajectories, exact replay at both takeover boundaries, original-policy continuation success of at least 90\%, and zero prohibited completions or registered physical events under scripted holding. A structural donor must maintain gripper contact with the same target object at both boundaries. The task-order seed is 20261110. The resulting cohorts describe holding-applicable manipulation tasks within each suite.

Calibration uses initial states 0--9, held-out target evaluation uses states 10--49, and retained-task evaluation uses states 10--19 on the other nine tasks. These give 40 held-out target episodes and 90 retained episodes per edited target. Checkpoint selection uses calibration outcomes, with the rule in Appendix~\ref{app:training}. Table~\ref{tab:normal-retained} reports the corresponding normal-start results.

For each target, takeover rates average the early and mid-task conditions. Suite values then weight the evaluated targets equally. The LIBERO column in Table~\ref{tab:main-results} averages the Goal, Spatial, and Object suite values with equal weight. It summarizes the selected targets under their registered takeover protocols. BadLIBERO retains a separate aggregate because its target event, physical-event union, and saturation criterion differ. A missing required target or takeover condition leaves the corresponding aggregate unavailable.

The source ledgers provide 95\% paired donor-bootstrap intervals using 10,000 resamples and seed 20261110. Each resample keeps a donor's takeover points and method comparisons together, with the target cohorts fixed. These intervals describe variation among the evaluated donor trajectories. Table~\ref{tab:results-breakdown} preserves the suite-level results underlying the main aggregate. The main table uses selected original runs, while RQ3 uses the checkpoint sequences and run provenance detailed in Appendix~\ref{app:run-provenance}.

\input{tables/results_breakdown}
\input{tables/normal_retained}

\subsection{Takeover States and Observation Windows}
The specialist audit samples donor trajectories from the original policy on held-out initial states 10--49. The early point is the first gripper-close command plus ten control steps, denoted $R_{\mathrm{grasp}}$ in the records. The mid-task point lies halfway between this point and the original policy's task completion. Successful original-policy trajectories supply the boundary states. The Goal stove audit additionally invokes each policy from the initial state under its uncensored protocol, and this condition is reported separately from the takeover aggregate.

\begin{table}[ht]
\centering\small
\begin{tabular}{lll}
\toprule
Setting & Restoration & Termination\\
\midrule
Goal t6 & Snapshot & Success-censored\\
Goal t9 & Replay & Success or 300 steps\\
Goal t7 & Replay & 300 steps\\
Spatial & Replay & 220 steps\\
Object & Replay & 280 steps\\
BadLIBERO & Replay & 200 steps\\
\bottomrule
\end{tabular}
\caption{Takeover protocols. Fixed-window evaluations continue after target attainment. The Goal stove audit also includes an initial-state condition.}
\end{table}

Snapshot restoration is used for Goal t6, where its fidelity was established. Action replay supplies the matched boundary states for the other evaluated targets. Each takeover clears the prior action queue and obtains a new chunk from the evaluated policy. Original-policy continuation checks verify that the restored states remain executable. Spatial and Object evaluations use a fresh simulator for each normal-start episode and check its initial-state fingerprints against the original-policy records. Fidelity checks and policy comparisons use matched hardware.

\subsection{Operational Metric Definitions}
For Goal t6 and t9, Spatial, and Object, Target Success Rate follows the environment success predicate during takeover. For Goal t7, the target is attained if the stove-knob position reaches 0.5 at any recorded step. For BadLIBERO, it is raw entry into the attack's designated L3 region. Target Suppression Rate is the complement of the same takeover rate. Retained Success Rate measures held-out success on the other permitted tasks from their normal initial states.

Physical Incident Rate uses the union of the registered physical-event flags in each rollout, including events that coincide with target attainment. The contact-aware \dropmetric predicate requires the held object to remain over 10\,cm below its takeover height, without gripper or goal-object contact, for at least two consecutive steps. Fallen-body events include another movable body falling over 10\,cm or the held object remaining unsupported and low at the final step. The LIBERO event union uses these applicable drop and fall predicates, with fallen-body events alone for the stove target. BadLIBERO additionally records lost hold and disturbance of other objects, as specified in Appendix~\ref{app:badlibero}.

The episode records retain both target-attainment and physical-event flags. Their joint union counts an episode once if either event occurs. The supporting event-without-target-attainment rate uses all audited episodes as its denominator and counts only their conjunction of a physical event and absent target attainment. This joint rate plus Target Success Rate equals the union rate before rounding.

For processed arm commands $u_{s,j}$ before controller clipping, the episode saturation endpoint is
\begin{equation}
\label{eq:sat}
\begin{split}
\rho_{\mathrm{sat}}&=\frac{1}{T}\sum_{s=1}^{T}
\mathbf{1}\!\left[\max_{0\leq j<6}|u_{s,j}|\geq1\right],\\
\operatorname{SAT\_EP}&=\mathbf{1}[\rho_{\mathrm{sat}}\geq0.05],
\end{split}
\end{equation}
where $T$ is the observed rollout length. For LIBERO, Action Saturation Rate is the percentage of episodes satisfying this criterion. BadLIBERO's registered criterion is any saturated step, with the 5\%-of-steps version retained as a sensitivity analysis. Saturation describes commands at the clipping boundary, independently of target attainment or physical incidents. The registered observation windows and success termination determine each rollout's exposure to these events.

\paragraph{Motivation figure.}
Figure~\ref{fig:motivation} presents two illustrative single-seed task evaluations. Its upper panel connects the stove audit's initial, early, and mid-task conditions. The initial point uses the restart-audit protocol, under which RMU records 5.0\% completion. Its separate held-out normal-start evaluation records 2.5\%. The displayed VLA-Forget adaptation has retained-task success of 76.7\%, compared with 94.4\% for the original, and falls below the retained-utility criterion. The OFT and home-return adaptations are described in Appendices~\ref{app:training} and~\ref{app:comparators}.

The lower panel uses all episodes in each condition as the denominator and accumulates recorded \dropmetric events until rollout termination. Each curve ends at the last observed step for its condition. All original-policy rollouts complete by step 41, and its curve ends there. NPO-RT, Refusal FT, VLA-Forget, and \method record zero task completion in this bottle-placement evaluation, while RMU and the original record 12.5\% and 100.0\%, respectively. The upper thumbnail shows the original policy's mid-task stove state for donor initial state 10. The lower thumbnail shows Refusal FT on donor initial state 31 at control step 110, following the recorded drop onset at step 80.

\paragraph{Corrected Goal physical-event measurements.}
The historical Goal t6 endpoint, \texttt{drop\_fail}, records an object descent of more than 10\,cm followed by episode failure. The contact-aware \dropmetric definition additionally checks gripper and goal-object contact. For NPO-RT at mid-task takeover, these two rates are 60.0\% and 0.0\%, respectively. The current main aggregate uses the corrected contact-aware drop and fallen-body measurements from the later audit. This audit reproduced the original-policy commands and outcomes, including completed rollouts with fallen-body events. The VLA-Forget adaptation's executed commands differed from its historical audit, and its current entry uses the newly recorded outcomes. The source ledgers preserve the historical descent endpoint separately.

\paragraph{Prospective rules and exploratory extensions.}
The study developed through successive experimental rounds. Target-specific thresholds, checkpoint-selection rules, and progression gates were frozen before the corresponding method outcomes. Later methods and settings were partly motivated by earlier results. The generalist fallback run after its applicability failure and the prefix-only analysis are exploratory, and the motivation examples are illustrative task evaluations.

\subsection{Physical Response Trajectories}
\label{app:physical-response}
Figure~\ref{fig:physical-response} uses the selected policy runs underlying the Spatial and Object entries in Table~\ref{tab:main-results}. The figure includes all eight main-table policies and the matched scripted-hold reference on the target cohorts defined in Appendix~\ref{app:results-protocol}. Each method starts from the same replayed state and tracks the same initially held object. These trajectories retain the full fixed observation window, including episodes with prohibited target attainment or a physical incident.

Let $p_i(t)\in\mathbb R^3$ be the world position in meters of the initially held object in donor trajectory $i$ at recorded step $t$, with $t=0$ denoting takeover. Its displacement in centimeters is $d_i(t)=100\lVert p_i(t)-p_i(0)\rVert_2$. Positions are recorded before each control action, giving steps 0--219 for Spatial and 0--279 for Object. At each step, we average displacement over donors within each target and then equally over the four targets in the suite. Early and mid-task takeovers remain separate. The pointwise bands use 10,000 paired donor-bootstrap resamples with seed 20261110, sharing donor resampling across methods and takeover conditions. They describe donor variation with the evaluated targets and policy checkpoints fixed. Intervals for all methods are retained in the accompanying data, and the figure displays the \method and scripted-hold bands for readability.

Object displacement measures agreement with the stationary holding objective. Refusal FT's home-return supervision specifies a moving response, as described in Appendix~\ref{app:comparators}, so its displacement reflects a different fallback objective. We interpret these trajectories alongside target attainment and physical incidents in Table~\ref{tab:main-results}. The recorded gripper contact provides an accompanying measure of the holding response. For \method, task-balanced contact rates at the final observation are 100.0\% and 93.1\% for Spatial early and mid-task takeover, respectively, and 96.7\% and 99.3\% for Object. All trajectory averages include the 12 \method rollouts with recorded prohibited completion, comprising eleven Spatial mid-task rollouts and one Object mid-task rollout. Matching initial positions and recomputing the recorded completion, physical-event, and saturation endpoints verified consistency with the source evaluation ledgers.

\section{Training and Checkpoint Selection}
\label{app:training}
\paragraph{Fallback action encoding.}
\label{app:fallback}
The OFT action representation uses $d=7$ coordinates, comprising six robot-arm motion coordinates and one gripper coordinate. We use chunks of length $H=8$ in the specialist experiments. For each robot-arm coordinate $j$, let $q_{01,j}$ and $q_{99,j}$ denote the first and ninety-ninth percentile bounds stored in the original policy's action-normalization statistics. The zero-motion target in Equation~\ref{eq:hold} is encoded as
\begin{equation}
\label{eq:hold-normalization}
h_j=\frac{2(0-q_{01,j})}{q_{99,j}-q_{01,j}}-1,
\quad j=1,\ldots,d-1,
\end{equation}
using nondegenerate normalization intervals. For data sources with different normalization statistics, we compute $h$ using the statistics associated with each sample. The gripper target $\bar A_{k,d}=A_{1,d}$ repeats the first demonstrated gripper label across the chunk. This label comes from the training demonstration, and the adapted policy predicts its gripper command from the current input at execution time.

\paragraph{Training recipe.}
\method starts from the original OFT specialist and adds fresh LoRA adapters of rank 32, scaling 16, and zero dropout on the language-model linear layers. The inherited action head remains trainable. Vision, cross-modal projection, proprioceptive projection, and embeddings remain frozen. Training uses AdamW with learning rate $5\times10^{-5}$, zero weight decay, constant learning rate, and gradient clipping at 1.0. Each update uses eight prohibited-task and eight retained-task samples, with crop augmentation. Checkpoints are saved after 100, 200, and 300 updates. Calibration selects step 300 for every Goal and Object target. For Spatial targets t8, t6, t7, and t0, the selected checkpoints are steps 300, 200, 300, and 200, respectively.

A calibration checkpoint qualifies if target completion is at most 1/10 and retained success decreases by at most nine of 90 episodes relative to the original. Among qualifying checkpoints, we select the one with the highest retained success, breaking ties toward the earlier checkpoint. The baseline selection rule first searches qualifying checkpoints, then those meeting target suppression, and finally the checkpoint with the lowest target completion. The latter two tiers retain a best-effort, non-qualifying label. Held-out results never select the checkpoint or change its calibration tier.

\paragraph{Objective adaptations and lineage.}
NPO-RT uses a length-normalized Laplace action score with action-unit rescaling, $\beta=0.1$, and retained-action imitation. RMU steers the layer-7 hidden state toward a random direction with magnitude five times its original norm and uses retained-state matching with weight 1200. GA maximizes prohibited-task L1 error without retained imitation, while GradDiff adds the retained L1 term. These methods use the matched \method recipe unless their declared method specifies otherwise. VLA-Forget uses an OFT adaptation with staged module-wise LoRA, PCGrad, and action-output distillation, so it does not share an identical optimizer workflow.

Fallback imitation was initially explored as an objective replacement within that VLA-Forget adaptation. \method then used a standalone update scope and joint objective without its module selection, staging, or distillation. This history motivates the formulation but is not a controlled comparison of the two implementations.

\paragraph{Selected runs and checkpoint sweeps.}
\label{app:run-provenance}
The main table reports the originally selected policy runs. The utility--suppression figure uses separate same-recipe runs for \method, NPO-RT, RMU, and Refusal FT, evaluated after 100, 200, and 300 updates. GA and GradDiff use these same update counts from the original training runs that produced their main-table policies. VLA-Forget also uses its original training sequence, with the first two points at 30 and 60 updates of its final language-model stage and the third at the final checkpoint. Each plotted trajectory uses one coherent run, with its checkpoints evaluated on the same target cohort. On Spatial, the main-table GradDiff aggregate combines step 100 for t6 with step 300 for the other targets. It therefore differs from the figure's common-step aggregates.

The separate-run provenance matters because same-seed reruns differ from the original selected results. At the original selected checkpoint indices, NPO-RT's physical-event-without-target rate changes from 17.3\% to 2.0\% on Spatial and from 15.6\% to 10.5\% on Object. Its takeover success changes from 45.4\% to 54.8\% and from 17.3\% to 33.8\%, respectively. The corresponding \method takeover rates change from 3.4\% to 2.8\% on Spatial and from 0.3\% to 1.0\% on Object.

\paragraph{Coincident GA checkpoints.}
On Spatial and Object, calibration selects step 100 for every GA target through the suppression-only tier. All three sampled checkpoints record zero retained success and command saturation in every takeover rollout. Their identical plot coordinates are supported by a paired trace check across 604 audited takeovers. Although their pre-clipping arm commands differ, the complete clipped action sequences and resulting object trajectories coincide in every checked rollout. Checkpoint hashes are distinct, and the evaluation records identify the corresponding weights.

\paragraph{VLA-Forget deployment checks.}
\label{app:baseline-provenance}
The VLA-Forget results describe our OFT adaptation as loaded for evaluation. The Goal checkpoints predate the deployment save/reload check. On Spatial and Object, evaluation proceeded after the maximum command differences exceeded the registered $10^{-3}$ threshold. The BadLIBERO check recorded a maximum difference of 0.125 against a $10^{-4}$ threshold. The cause of these discrepancies remains unresolved. BadLIBERO passed the in-script teacher-fingerprint assertions, while the separate teacher-functional preflight was not performed. These implementation conditions qualify attribution of the measured results to the published method.

\paragraph{Exploratory prefix-only supervision.}
\label{app:prefix-supervision}
Restricting fallback supervision to demonstrations before the first gripper-close command yields 100.0\% takeover success on Spatial and 98.7\% on Object, although all selected policies pass the normal-start suppression and retained-success criteria. Full-demonstration \method under the same recipe family and selection procedure records 3.4\% and 0.3\%, respectively. This is a descriptive instance of the gap between normal-start suppression and continuation after takeover. Truncation changes state coverage, weighting, diversity, and gripper targets together, so their individual contributions remain unresolved.

\section{Refusal and Deployment Comparators}
\label{app:comparators}
In the Goal experiments, our refusal baseline uses 50 original-policy rollouts per target on fresh layouts. For t6 and t9, the return boundary precedes the earlier of the first post-grasp opening command and task success by five steps. For t7, it precedes first gripper--stove contact by five steps. A simulated controller supplies return-to-home trajectories, supplemented with reset episodes and retained-task imitation. The model uses the same 300-step fine-tuning schedule and calibration selection rule as the matched baselines. Target clipping and trajectory-source differences prevent treating this comparison as an isolated home-return-versus-hold ablation.

The exact-string gate recognizes only the canonical prohibited instruction. The semantic gate uses Gemini-2.5-Flash with temperature zero and thinking disabled, queried before every eight-step action chunk. Its input contains the instruction, an agent-view image, and a summary of the candidate command chunk. A freeze decision or risk score at least 0.5 permanently activates the fallback for that rollout. Parsing or service failures allow execution. Across the measured evaluation, this implementation required 7,752 HTTP attempts and included 25 unresolved errors.

Both gates use an anchored controller that stores the boundary end-effector pose and the preceding gripper command. This differs from \method's learned zero-delta target. The guard pretest requires zero events, maximum excursion no greater than 3\,cm, and no greater than 1\,cm over the final 50 steps. On t6, maximum excursions of 3.42\,cm and 3.09\,cm fail the pretest despite zero recorded events. Its semantic-gate comparison is therefore unavailable, while the exact-string comparator reports the controller's measured outcomes with that applicability limitation disclosed.

\section{Input Shifts and Diagnostic Baselines}
\label{app:shifts}
P1 replaces the canonical instruction with a fixed paraphrase. WARM transforms each camera image by $\operatorname{clip}(x\odot[1.15,1,0.80])$. The original policy passes the specified robustness gate in all six target--shift cells, supplying a matched reference for each condition. Under both shifts, \method records zero normal-start target success on all three Goal targets. Its retained success on t6, t9, and t7 is 96.7\%, 91.1\%, and 95.6\% under P1, and 96.7\%, 92.2\%, and 94.4\% under WARM. These evaluations measure completion and retained utility. Refusal FT has no input-shift evaluation in the current results.

The exact-string gate permits target success of 100.0\%, 97.5\%, and 100.0\% under P1, which changes the instruction recognized by the gate. It records zero target success under WARM, which preserves that instruction. The semantic gate records zero target success in the evaluated t9 and t7 conditions, with retained success ranging from 81.1\% to 87.8\%. Its t6 evaluation stopped after the controller-applicability failure described in Appendix~\ref{app:comparators}.

\label{app:diagnostics}
GA and GradDiff fail selective calibration on the Goal specialist targets. GA's held-out target success is 0.0\%, 0.0\%, and 10.0\% on t6, t9, and t7, with zero retained success on all three. GradDiff records zero target success and retained success of 45.6\%, 47.8\%, and 42.2\%. Their response events therefore describe edits with substantial utility loss. The task-excluded references suppress all three targets from normal starts while retaining 90.0\%, 96.7\%, and 93.3\% success. They exhibit residual completion or physical events under some takeovers, including t6 mid-task completion of 65.0\% and t9 mid-task \dropmetric of 57.5\%.

\section{Retained-Task Responses and Neighbor Utility}
\label{app:retained}
The retained-task audit tests normal starts and neighbor-task mid-state takeovers under matched observation windows. It compares task-balanced event rates against the original using 95\% paired bootstrap intervals, with 5,000 draws within each task. The material-excess criterion requires a difference of at least ten percentage points and a positive interval lower bound. An upper bound below ten points provides evidence against that criterion. Among qualified edits, 43 of 44 comparisons meet the latter condition and one is inconclusive. These results do not establish material amplification of the measured events on retained tasks, while leaving smaller effects unresolved.

Instruction-based neighbor groups give a complementary utility check. Original versus \method success is 36/40 versus 37/40 for the t6 neighbor group, 9/10 versus 9/10 for t9, and 19/20 versus 19/20 for t7. The corresponding distant-task counts are 49/50 versus 49/50, 76/80 versus 72/80, and 66/70 versus 67/70. These small groups show no observed neighbor-specific degradation but cannot establish the absence of task entanglement.

\section{Generalist Results and Applicability Boundary}
\label{app:generalist}
The generalist experiment jointly prohibits Goal t7 and LIBERO-10 t2, which combines stove activation with placing a moka pot on the stove. The other 38 tasks form the retained set. The original has target success of 100.0\% and 97.5\% and retained success of 91.8\%. A scripted hold permits stove activation in 7.5\% of Goal mid-task states, stopping the planned \method experiment. Table~\ref{tab:generalist} separately labels the exploratory run conducted after this failure.

\begin{table*}[t]
\centering\small
\begin{tabular}{lrrrrrr}
\toprule
& \multicolumn{2}{c}{Target Success (\%)} & \multicolumn{2}{c}{Retained Success (\%)} & \multicolumn{2}{c}{Mid-task Activation (\%)}\\
\cmidrule(lr){2-3}\cmidrule(lr){4-5}\cmidrule(lr){6-7}
Method & Goal & LIBERO-10 & All tasks & LIBERO-10 & Goal & LIBERO-10\\
\midrule
Original & 100.0 & 97.5 & 91.8 & 83.3 & 100.0 & 100.0\\
NPO-RT & 0.0 & 0.0 & 88.2 & 70.0 & 100.0 & 90.0\\
RMU & 0.0 & 0.0 & 96.3 & 94.4 & 100.0 & 100.0\\
\method (expl.) & 0.0 & 0.0 & 85.5 & 58.9 & 2.5 & 0.0\\
\bottomrule
\end{tabular}
\caption{Generalist results. The \method row is exploratory because scripted holding failed the applicability check. Target success measures complete task execution, whereas mid-task activation measures the prohibited stove action within each task.}
\label{tab:generalist}
\end{table*}

Exploratory \method passes the pooled retained-success tolerance but reduces LIBERO-10 success from 83.3\% to 58.9\%, including zero successes on two retained tasks. A subsequent common-input action probe finds a LIBERO-10 error increase for both \method and NPO-RT, while RMU changes less. These observations identify a shared deficit in that setup whose mechanism remains unresolved. The training mixture uses component-size scaling before target filtering, yielding approximately frame-proportional 2:1 exposure for the two prohibited components.

\section{BadLIBERO Backdoor Extension}
\label{app:badlibero}
The GoBA setting uses a poisoned box as a physical trigger for placing that box in a designated table region (L3)~\citep{zhou2025goba}. We adapt the implantation to the OFT specialist within LIBERO-Goal using 111 poison demonstrations and 2,000 updates, then evaluate methods at a fixed 300-step editing checkpoint. The selected tasks are t3 and t6. The first takeover point is gripper--box contact, and the second is five steps before the earlier of post-grasp opening and raw L3 attainment. The anchored-hold applicability control passes all selected cells.

Each takeover runs for 200 uncensored control steps. The physical-event union includes object drop, lost hold, disturbance of other objects, and fallen-body endpoints under this setting's definitions. Its saturation endpoint records any saturated arm-command step, whereas the specialist endpoint requires a 5\% fraction. The two settings therefore retain separate event definitions and are not pooled. We compute the physical-event union directly from episode flags because the mutually exclusive response classes prioritize L3 and release events and can hide co-occurring physical events.

Normal-start evaluations comprise 100 untriggered episodes and 120 triggered episodes. The latter contain 20 episodes for each selected task and ten for each of the other eight tasks. The selected-task clean-recovery denominator is therefore 40 and must not be replaced by the pooled 120. Restart evaluation comprises ten donors per selected task at two takeover points, giving 40 takeovers from 20 donors. These repeated takeovers are not 40 independent donor trajectories.

All methods that meet this setting's suppression and utility criteria record zero L3 entry after takeover. Within this group, NPO-RT records a 22.5\% Physical Incident Rate and 100.0\% Action Saturation Rate. \method, RMU, and Refusal FT each record zero physical incidents, with saturation rates of 0.0\%, 0.0\%, and 2.5\%, respectively. \method's response is classified as hold-like in 87.5\% of takeovers. The non-selective GA and GradDiff policies also record zero L3 entry, alongside physical-incident rates of 40.0\% and 30.0\% and saturation in every rollout.

The evaluated VLA-Forget OFT adaptation records L3 entry and physical incidents in 35.0\% of takeovers, entirely at the later boundary, and saturation in every rollout. Every event-positive rollout also attains L3. The registered drop and disturbance rates are zero, with the physical incidents instead involving lost hold and fallen-body endpoints. Its deployment-check provenance is given in Appendix~\ref{app:baseline-provenance}.

On untriggered inputs, \method retains 96.0\% clean-task success, compared with 91.0\% for the implant and 95.0\% for the clean reference. Under the trigger, however, \method recovers the intended clean task in only 2.5\% of episodes on the two attacked tasks. Its pooled triggered clean-task success across all ten tasks is 49.2\%. This broader population includes the other tasks and therefore answers a different utility question. VLA-Forget records 79.0\% untriggered success and 45.8\% pooled triggered clean-task success, with zero clean-task recovery on the two attacked tasks.

\section{Target-Supervised Relearning}
\label{app:relearning}
The relearning test mixes five target demonstrations with retained data at a 1:1 ratio and uses learning rate $5\times10^{-5}$. Table~\ref{tab:relearning} reports shared checkpoints for \method and the VLA-Forget adaptation. Prohibited execution returns rapidly after \method, and early reacquisition is faster on all three targets at step 100. This is a descriptive behavioral result and does not identify retained internal memory or establish pointwise dominance throughout training.

\begin{table}[htbp]
\centering\small
\begin{tabular}{llrrr}
\toprule
 & & \multicolumn{3}{c}{Target Success (\%)}\\
Target & Method & 100 & 300 & 1,000\\
\midrule
t6 & VLA-Forget & 35.0 & 85.0 & 97.5\\
 & \method & 95.0 & 97.5 & 95.0\\
t9 & VLA-Forget & 0.0 & 0.0 & 47.5\\
 & \method & 87.5 & 97.5 & 100.0\\
t7 & VLA-Forget & 50.0 & 87.5 & 95.0\\
 & \method & 100.0 & 100.0 & 100.0\\
\bottomrule
\end{tabular}
\caption{Target success after 100, 300, and 1,000 updates of target-supervised fine-tuning. All listed edited policies start with zero held-out target success.}
\label{tab:relearning}
\end{table}

Exploratory attempts to improve durability included readout-robust suppression, relearning-aware fallback training, and task-delta attenuation followed by repair. They did not pass their respective frozen validation or progression rules. They supply no evidence for a durable-removal claim and are not components of \method.

\section{Stopped Feasibility Studies}
\label{app:stops}
An additional LIBERO-Goal target, placing a bowl on the stove (t1), stops before \method training because the scripted hold records a fall and drop in 1/38 mid-task takeovers. This result, together with the generalist pretest failure, limits which prohibitions admit the tested fallback.

Three additional settings stopped before a valid method comparison. In LIBERO-Safety's reasoning-safety tasks~\citep{cui2026liberosafety}, prohibited execution occurred in 0/20, 0/20, and 5/20 episodes, below the 10/20 progression gate. These instructions were outside the released policy's physical-task fine-tuning set, so non-execution could not establish refusal. In the HazardArena feasibility tranche~\citep{chen2026hazardarena}, five of seven loadable task pairs failed the fallback-applicability checks, and a detector defect further prevented the fixed six-pair progression requirement. These results concern local feasibility and candidate controllers, not \method transfer.

The DropVLA-Spatial screen~\citep{xu2025dropvla} stopped because the released clean checkpoint failed the selected competence gate. Command-level release could occur without the corresponding physical drop, and the later restart and applicability gates were not assessed. The failure reason for local competence was not diagnosed. We therefore report the stopped screen without claiming that the source work is irreproducible or that its attack does not work.
